# Supplementary material for: Prediction of triple point fermions in simple half-Heusler topological insulators
Source: arXiv:1706.00200 source file (2017-06-01)
Supplement: Supplementary file 1 [file supplementary.pdf]

# Supplementary Materials for
# "Prediction of triple point fermions in simple half-Heusler topological insulators"

Hao Yang,[1] Jiabin Yu,[2] Stuart S. P. Parkin,[1] Claudia Felser,[3] Chao-Xing Liu,[2] and Binghai Yan[4,*]

[1] *Max Planck Institute of Microstructure Physics, Weinberg 2, 06120 Halle, Germany*
[2] *Department of Physics, the Pennsylvania State University, University Park, PA, 16802*
[3] *Max Planck Institute for Chemical Physics of Solids, 01187 Dresden, Germany*
[4] *Department of Condensed Matter Physics, Weizmann Institute of Science, Rehovot, 7610001, Israel*

The outline is in the following.

1. General Conditions for Existence of Triple Points.

2. Triple Points in a Chosen Parameter Region.

3. Kane Model Parameter Choices for Surface States.

4. Bands structure of LuPtBi, LuAuPb and LuPdBi.

5. *Ab inito* calculations of surface states for YPtBi and LaPtBi.

## I. General Conditions for Existence of Triple Points

For half-Heusler materials without any external effects like magnetic field or distortion, their space group and point group are $F\bar{4}3m$ group and $T_d$ group respectively.[1,2] Therefore, their physics around $\Gamma$ point near Fermi level is commonly described by six-band Kane model[3]. With bases to be $|\Gamma_6, \frac{1}{2}\rangle$, $|\Gamma_6, -\frac{1}{2}\rangle$, $|\Gamma_8, \frac{3}{2}\rangle$, $|\Gamma_8, \frac{1}{2}\rangle$, $|\Gamma_8, -\frac{1}{2}\rangle$ and $|\Gamma_8, -\frac{3}{2}\rangle$, the standard six-band Kane model is[3]

$$H_{Kane}(\mathbf{k}) = \left(\begin{array}{c|c} H_{\Gamma_6}(\mathbf{k}) & V \\ \hline V^\dagger & H_{\Gamma_8}(\mathbf{k}) \end{array}\right), \tag{1}$$

where

$$\begin{aligned} V = &\frac{P}{\sqrt{6}}\begin{pmatrix} -\sqrt{3}k_+ & 2k_z & k_- & 0 \\ 0 & -k_+ & 2k_z & \sqrt{3}k_- \end{pmatrix} \\ &+\frac{B_{8v}^+}{\sqrt{6}}\begin{pmatrix} \sqrt{3}k_-k_z & 2ik_xk_y & k_+k_z & 0 \\ 0 & k_-k_z & 2ik_xk_y & \sqrt{3}k_+k_z \end{pmatrix} \\ &+\frac{B_{8v}^-}{3\sqrt{2}}\begin{pmatrix} 0 & \sqrt{3}K^2 & 0 & k_\parallel^2 - 2k_z^2 \\ -k_\parallel^2 + 2k_z^2 & 0 & -\sqrt{3}K^2 & 0 \end{pmatrix} \end{aligned}, \tag{2}$$

$$H_{\Gamma_6}(\mathbf{k}) = (E_c + \beta_c k^2)\mathbb{1}_2 \tag{3}$$

with $\mathbb{1}_2$ to be the $2\times 2$ identity matrix,

$$H_{\Gamma_8}(\mathbf{k}) = H_0(\mathbf{k}) + H_C(\mathbf{k}) \tag{4}$$

with

$$\begin{aligned} H_0(\mathbf{k}) = &\tfrac{4}{15}(J_x^2 + J_y^2 + J_z^2)h_0 + \tfrac{1}{3}(2J_z^2 - J_x^2 - J_y^2)h_1 \\ &+\tfrac{1}{\sqrt{3}}(J_x^2 - J_y^2)h_2 + \tfrac{2}{\sqrt{3}}J_{xy}h_3 + \tfrac{2}{\sqrt{3}}J_{zx}h_4 + \tfrac{2}{\sqrt{3}}J_{yz}h_5 \end{aligned} \tag{5}$$

and

$$H_C(\mathbf{k}) = \frac{2}{\sqrt{3}}C(k_xV_x + k_yV_y + k_zV_z). \tag{6}$$

Here we have $h_0 = E_v - \beta_c\gamma_1 k^2$, $h_1 = \beta_c\gamma_2(2k_z^2 - k_\parallel^2)$, $h_2 = \sqrt{3}\beta_c\gamma_2 K^2$, $h_3 = 2\sqrt{3}\beta_c\gamma_3 k_xk_y$, $h_4 = 2\sqrt{3}\beta_c\gamma_3 k_xk_z$, and $h_5 = 2\sqrt{3}\beta_c\gamma_3 k_yk_z$. $J_i$'s are angular momentum matrices for spin 3/2, $J_{ij} = \frac{1}{2}\{J_i, J_j\}$, $V_x = \frac{1}{2}\{J_x, J_y^2 - J_z^2\}$, $V_y = \frac{1}{2}\{J_y, J_z^2 - J_x^2\}$, $V_z = \frac{1}{2}\{J_z, J_x^2 - J_y^2\}$, $\beta_c = \hbar^2/(2m')$, $m'$ is the effective mass of $\Gamma_6$ bands near $\Gamma$ point, $k^2 = k_x^2 + k_y^2 + k_z^2$, $k_\parallel^2 = k_x^2 + k_y^2$, $K^2 = k_x^2 - k_y^2$ and $k_\pm = k_x \pm ik_y$.

**In this work, $\gamma_2 \neq 0$ and $\gamma_3 \neq 0$ are always assumed. Moreover, $\beta_c > 0$ and $E_c < E_v$ are assumed, which means $\Gamma_6$ bands are lower than $\Gamma_8$ bands and is commonly ture for half-Heusler materials with inverted band structure.**[4–7]

For symmorphic triple points(TPs) to exist, $C_{3v}^*$ spin double group is typically essential.[8] The character table of $C_{3v}^*$ spin double group is shown in Tab.I.

| $C_{3v}^*$ | E | R | $C_3$,$C_3^2$R | $C_3^2$, $C_3$R | $3\sigma_v$ | $3\sigma_v$R |
|---|---|---|---|---|---|---|
| $\Lambda_1$ | 1 | 1 | 1 | 1 | 1 | 1 |
| $\Lambda_2$ | 1 | 1 | 1 | 1 | -1 | -1 |
| $\Lambda_3$ | 2 | 2 | -1 | -1 | 0 | 0 |
| $\Lambda_4$ | 1 | -1 | -1 | 1 | i | -i |
| $\Lambda_5$ | 1 | -1 | -1 | 1 | -i | i |
| $\Lambda_6$ | 2 | -2 | 1 | -1 | 0 | 0 |

TABLE I. Character Table of Spin Double Group $C_{3v}^*$ [9]

Inside $T_d$ group, there are 4 different $C_{3v}$ subgroups with principle axis (axis of $C_3$) along (111),($\bar{1}$11),(1$\bar{1}$1) and (11$\bar{1}$), which can be related by $S_4^z$ operation. That means we only need to consider one $C_{3v}$ group, and the one chosen

to be studied here is $C_{3v}$ with $C_3$ along (111) direction, noted as $C_{3v}^{(111)}$. Mirror planes of $C_{3v}^{(111)}$ are $(1\bar{1}0)$, $(\bar{1}01)$ and $(01\bar{1})$ planes.

For $\Gamma_6$ and $\Gamma_8$ bases, the generators of $C_{3v}^{(111)}$ are represented as

$$C_3(111) \doteq \begin{pmatrix} \exp(-i\frac{S_x+S_y+S_z}{\sqrt{3}}\frac{2\pi}{3}) & 0 \\ 0 & \exp(-i\frac{J_x+J_y+J_z}{\sqrt{3}}\frac{2\pi}{3}) \end{pmatrix}$$

$$\pi_{1\bar{1}0} \doteq \begin{pmatrix} \exp(-i\frac{S_x-S_y}{\sqrt{2}}\pi) & 0 \\ 0 & -\exp(-i\frac{J_x-J_y}{\sqrt{2}}\pi) \end{pmatrix}$$

, where $S_i = \sigma_i/2$ and $\sigma_i$'s are Pauli matrices. Based on that, we can group $\Gamma_6$ and $\Gamma_8$ bases into those three irreducible representations. Wave functions for each irreducible representation in bases $|\Gamma_6, 1/2\rangle$, $|\Gamma_6, -1/2\rangle$, $|\Gamma_8, 3/2\rangle$, $|\Gamma_8, 1/2\rangle$, $|\Gamma_8, -1/2\rangle$ and $|\Gamma_8, -3/2\rangle$ are shown below:

$\Lambda_4$:

$$\psi_{\Lambda_4} = N_4\left(0, 0, \frac{1-i}{\sqrt{2}}, \frac{\sqrt{2}-i}{\sqrt{3}}, i\left(\frac{1}{\sqrt{6}}+\frac{1}{\sqrt{3}}\right) - \sqrt{\frac{1}{6}\left(3-2\sqrt{2}\right)}, 1\right) \tag{7}$$

$\Lambda_5$:

$$\psi_{\Lambda_5} = N_5\left(0, 0, \frac{-1+i}{\sqrt{2}}, -\frac{\sqrt{2}+i}{\sqrt{3}}, i\sqrt{\frac{1}{6}\left(3-2\sqrt{2}\right)} - \frac{1}{\sqrt{3}} - \frac{1}{\sqrt{6}}, 1\right) \tag{8}$$

$\Lambda_6$:

$$\psi_{\Lambda_6,1} = \frac{1}{\sqrt{6}}\left(0, 0, -1-i, i\sqrt{3}, 0, 1\right), \psi_{\Lambda_6,2} = \frac{1}{\sqrt{6}}\left(0, 0, i, 0, \sqrt{3}, 1+i\right) \tag{9}$$

$$\phi_{\Lambda_6,1} = (1,0,0,0,0,0), \phi_{\Lambda_6,2} = (0,1,0,0,0,0) \tag{10}$$

,where $N_4$ and $N_5$ are normalization factors. Eq.9 and Eq.10 list two linearly independent sets of wavefunctions of $\Lambda_6$, and any linearly combination of them with same coefficients for both components can still give a $\Lambda_6$ irreducible representation of $C_{3v}^{*}$. Transform $H_{Kane}(\mathbf{k})$ into bases $(\psi_{\Lambda_4}, \psi_{\Lambda_5}, \psi_{\Lambda_6,1}, \psi_{\Lambda_6,2}, \phi_{\Lambda_6,1}, \phi_{\Lambda_6,2})$, and the transformed $H_{Kane}(\mathbf{k})$ along $k_x = k_y = k_z = k$ direction is represented as

$$\begin{pmatrix} E_{\Lambda_4}(k) & 0 & 0 & 0 & 0 & 0 \\ 0 & E_{\Lambda_5}(k) & 0 & 0 & 0 & 0 \\ 0 & 0 & E_v - 3k^2\beta_c(\gamma_1+2\gamma_3) & 0 & -\frac{2ik(P-iB_{8v}^{+}k)}{\sqrt{3}} & \frac{(1+i)k(P-iB_{8v}^{+}k)}{\sqrt{3}} \\ 0 & 0 & 0 & E_v - 3k^2\beta_c(\gamma_1+2\gamma_3) & \frac{(1+i)k(P-iB_{8v}^{+}k)}{\sqrt{3}} & \frac{2k(P-iB_{8v}^{+}k)}{\sqrt{3}} \\ 0 & 0 & \frac{2ik(P+iB_{8v}^{+}k)}{\sqrt{3}} & \frac{(1-i)k(P+iB_{8v}^{+}k)}{\sqrt{3}} & 3\beta_c k^2 + E_c & 0 \\ 0 & 0 & \frac{(1-i)k(P+iB_{8v}^{+}k)}{\sqrt{3}} & \frac{2k(P+iB_{8v}^{+}k)}{\sqrt{3}} & 0 & 3\beta_c k^2 + E_c \end{pmatrix} \tag{11}$$

, where $E_{\Lambda_4}(k) = E_v - k\left(3k\beta_c(\gamma_1 - 2\gamma_3) + C\sqrt{6}\right)$, $E_{\Lambda_5}(k) = E_v + k\left(\sqrt{6}C - 3k\beta_c(\gamma_1 - 2\gamma_3)\right)$. Diagonolizing it gives the energy dispersion of $H_{Kane}(\mathbf{k})$ along $k_x = k_y = k_z = k$:

$$\begin{aligned} E_{\Lambda_4}(k) &= E_v - k\left(3k\beta_c(\gamma_1 - 2\gamma_3) + C\sqrt{6}\right) \\ E_{\Lambda_5}(k) &= E_v + k\left(\sqrt{6}C - 3k\beta_c(\gamma_1 - 2\gamma_3)\right) \\ E_{\Lambda_6^-}(k) &= \tfrac{1}{2}\left(E_c + E_v - 3\beta_c k^2(\gamma_1 + 2\gamma_3 - 1) - \sqrt{\left[E_c - E_v + 3\beta_c k^2(\gamma_1 + 2\gamma_3 + 1)\right]^2 + 8k^2(P^2 + (B_{8v}^{+})^2k^2)}\right) \\ E_{\Lambda_6^+}(k) &= \tfrac{1}{2}\left(E_c + E_v - 3\beta_c k^2(\gamma_1 + 2\gamma_3 - 1) + \sqrt{\left[E_c - E_v + 3\beta_c k^2(\gamma_1 + 2\gamma_3 + 1)\right]^2 + 8k^2(P^2 + (B_{8v}^{+})^2k^2)}\right) \end{aligned} \tag{12}$$

, where $E_{\Lambda_6^{\pm}}(k)$ are both doubly degenerate.

Now, a transformation is made to make all quantity dimensionless : $\tilde{E} \equiv E/\varepsilon_0$, $\tilde{k} \equiv ka$, $\tilde{C} \equiv C/(\beta_c/a)$, $\tilde{B}^{\pm}_{8v} \equiv B^{\pm}_{8v}/\beta_c$ and $\tilde{P} \equiv P/(\beta_c/a)$, where $\varepsilon_0 \equiv \frac{\beta_c}{a^2}$ and $a$ is a positive parameters with unit of length.

Since $\tilde{E}_{\Lambda_6^-}(0) = \tilde{E}_c$ and $\tilde{E}_{\Lambda_6^+}(0) = \tilde{E}_v$, $\tilde{E}_{\Lambda_6^-}(k)$ is not involved in creating triple points (TPs) while $\tilde{E}_{\Lambda_6^+}(k)$ is. Therefore, TPs are created by band crossing between $\tilde{E}_{\Lambda_6^+}(k)$ and $\tilde{E}_{\Lambda_4}(\tilde{k})$ or $\tilde{E}_{\Lambda_6^+}(\tilde{k})$ and $\tilde{E}_{\Lambda_5}(\tilde{k})$. Since $\psi_{\Lambda_4} \propto \Theta\psi_{\Lambda_5}$, $\psi_{\Lambda_6,1} \propto \Theta\psi_{\Lambda_6,2}$ and $\phi_{\Lambda_6,1} \propto \Theta\phi_{\Lambda_6,2}$, we have $\tilde{E}_{\Lambda_4}(\tilde{k}) = \tilde{E}_{\Lambda_5}(-\tilde{k})$ and $\tilde{E}_{\Lambda_6^{\pm}}(\tilde{k}) = \tilde{E}_{\Lambda_6^{\pm}}(-\tilde{k})$, where $\Theta$ is time reversal symmetry operation. That means we only need to consider the band crossing situation between $\tilde{E}_{\Lambda_6^+}(\tilde{k})$ and $\tilde{E}_{\Lambda_4}(\tilde{k})$ and the band crossing condition between $\tilde{E}_{\Lambda_6^+}(\tilde{k})$ and $\tilde{E}_{\Lambda_5}(\tilde{k})$ can be obtained from time reversal symmetry.

Band crossing condition between $\tilde{E}_{\Lambda_6^+}(\tilde{k})$ and $\tilde{E}_{\Lambda_4}(\tilde{k})$ is

$$\tilde{E}_{\Lambda_4}(\tilde{k}) = \tilde{E}_{\Lambda_6^+}(\tilde{k}) \Leftrightarrow \tilde{k}\left(2\sqrt{6}\tilde{C} + 3\tilde{k}(\gamma_1 - 6\gamma_3 + 1)\right) + \tilde{E}_c - \tilde{E}_v + \sqrt{\left[\tilde{E}_c - \tilde{E}_v + 3\tilde{k}^2(\gamma_1 + 2\gamma_3 + 1)\right]^2 + 8\tilde{k}^2(\tilde{P}^2 + (\tilde{B}^{+}_{8v})^2\tilde{k}^2)} = 0 \tag{13}$$

That is equivalent to

$$\tilde{k}\left(2\sqrt{6}\tilde{C} + 3\tilde{k}(\gamma_1 - 6\gamma_3 + 1)\right) + \tilde{E}_c - \tilde{E}_v \leq 0 \;\&\; \tilde{k}\left(a_0 + a_1\tilde{k} + a_2\tilde{k}^2 + a_3\tilde{k}^3\right) = 0 \tag{14}$$

, where $a_0 = \sqrt{6}\tilde{C}(\tilde{E}_v - \tilde{E}_c)$, $a_1 = -6\tilde{C}^2 + 12\gamma_3\tilde{E}_c - 12\gamma_3\tilde{E}_v + 2\tilde{P}^2$, $a_2 = -3\sqrt{6}\tilde{C}\gamma_1 + 18\sqrt{6}\tilde{C}\gamma_3 - 3\sqrt{6}\tilde{C}$ and $a_3 = 36\gamma_1\gamma_3 - 72\gamma_3^2 + 36\gamma_3 + 2(\tilde{B}^{+}_{8v})^2$.

Eq.14 gives $\tilde{k} = 0$ solution, which is the 4-fold degenerate point at $\Gamma$ point instead of a TP. All other $\tilde{k} \neq 0$ solutions are TPs if $\tilde{E}_{\Lambda_5}(\tilde{k})$ does not cross with $\tilde{E}_{\Lambda_4}(\tilde{k})$ at those solution $\tilde{k}$ points.

The band crossing condition between $\tilde{E}_{\Lambda_5}(\tilde{k})$ and $\tilde{E}_{\Lambda_4}(\tilde{k})$ is

$$\tilde{E}_{\Lambda_4}(\tilde{k}) = \tilde{E}_{\Lambda_5}(\tilde{k}) \Leftrightarrow \tilde{C}\tilde{k} = 0 \tag{15}$$

, which means they only cross at $\Gamma$ point if $C \neq 0$. If $\tilde{C} = 0$, $\tilde{E}_{\Lambda_4}(\tilde{k}) = \tilde{E}_{\Lambda_5}(\tilde{k})$ would be always true and there would be no TPs. **Therefore, we need to assume $\tilde{C} \neq 0$ in order to have TPs.**

Based on the discussion above, we have a condition for a TP to exist at $\tilde{k}$:

$$\tilde{C} \neq 0 \;\&\; b_0 + b_1\tilde{k} + b_2\tilde{k}^2 \leq 0 \;\&\; a_0 + a_1\tilde{k} + a_2\tilde{k}^2 + a_3\tilde{k}^3 = 0 \;\&\; \tilde{k} \neq 0 \tag{16}$$

, where $b_0 = \tilde{E}_c - \tilde{E}_v$, $b_1 = 2\sqrt{6}\tilde{C}$ and $b_2 = 3(\gamma_1 - 6\gamma_3 + 1)$.

Condition listed in Eq.16 only allows at most three solutions, which means there are at most six TPs along one $C_3$ axis after taking time reversal symmetry in to consideration.

## II. Triple Points in a Chosen Parameter Region

To illustrate the physics, we choose this set of parameters:

| $\frac{E_v}{\varepsilon_0}$ | $\gamma_1$ | $\gamma_3$ | $\frac{P}{\beta_c/a}$ | $B^{+}_{8v}/\beta_c$ | $B^{-}_{8v}/\beta_c$ |
|---|---|---|---|---|---|
| 0 | 2 | $\frac{1}{2}$ | $\frac{5}{2}$ | 0 | 0 |

, where $\varepsilon_0 = \frac{\beta_c}{a^2}$, $a$ is a positive parameters with unit of length, $\tilde{E}_{cv} \equiv \frac{E_c - E_v}{\varepsilon_0} \in [-5, -0.5]$ and $\tilde{C} \equiv \frac{C}{\beta_c/a} \in [-0.3, -0.01]$. This is the parameter choice for the phase diagram shown in Fig.1g.

In this case,

| $b_0$ | $b_1$ | $b_2$ | $a_0$ | $a_1$ | $a_2$ | $a_3$ |
|---|---|---|---|---|---|---|
| $\tilde{E}_{cv}$ | $2\sqrt{6}\tilde{C}$ | 0 | $-\sqrt{6}\tilde{C}\tilde{E}_{cv}$ | $12.5 - 6\tilde{C}^2 + 6\tilde{E}_{cv}$ | 0 | 36 |

Under these conditions,

$$b_0 + b_1\tilde{k} + b_2\tilde{k}^2 \leq 0 \Leftrightarrow \tilde{k} \geq -\frac{b_0}{b_1}$$

Now, prove that all roots of $a_0 + a_1\tilde{k} + a_2\tilde{k}^2 + a_3\tilde{k}^3 = 0$ lie in $[-\frac{b_0}{b_1}, +\infty)$ for the parameter region we choose.

**Proof:**

Define $\tilde{k}_0 \equiv -\frac{b_0}{b_1}$.

(i)Prove $a_0 + a_1\tilde{k}_0 + a_2\tilde{k}_0^2 + a_3\tilde{k}_0^3 < 0$ for the parameter region we choose.

$$a_0 + a_1\tilde{k}_0 + a_2\tilde{k}_0^2 + a_3\tilde{k}_0^3 = -\frac{\tilde{E}_{cv}}{4\sqrt{6}\tilde{C}^3}\left(12\tilde{C}^4 + 25\tilde{C}^2 + 12\tilde{C}^2\tilde{E}_{cv} + 3\tilde{E}_{cv}^2\right)$$

. For the chosen parameter region, $-\frac{\tilde{E}_{cv}}{4\sqrt{6}\tilde{C}^3} < 0$ and $\left(12\tilde{C}^4 + 25\tilde{C}^2 + 12\tilde{C}^2\tilde{E}_{cv} + 3\tilde{E}_{cv}^2\right) > 0$, therefore

$$a_0 + a_1\tilde{k}_0 + a_2\tilde{k}_0^2 + a_3\tilde{k}_0^3 < 0$$

.

(ii)Prove $\frac{d}{d\tilde{k}}(a_0 + a_1\tilde{k} + a_2\tilde{k}^2 + a_3\tilde{k}^3) > 0$ for any $\tilde{k} < \tilde{k}_0$ and the parameter region we choose.

$$\frac{d}{d\tilde{k}}(a_0 + a_1\tilde{k} + a_2\tilde{k}^2 + a_3\tilde{k}^3) = -6\tilde{C}^2 + 6\tilde{E}_{cv} + 108\tilde{k}^2 + \frac{25}{2}$$

, which means the minimum of $\frac{d}{d\tilde{k}}(a_0 + a_1\tilde{k} + a_2\tilde{k}^2 + a_3\tilde{k}^3)$ is at $\tilde{k} = 0$. Since $-6\tilde{C}^2 + 6\tilde{E}_{cv} + 108\tilde{k}_0^2 + \frac{25}{2} > 0$ and $\tilde{k}_0 < 0$ in the chosen parameter region, we have $\frac{d}{d\tilde{k}}(a_0 + a_1\tilde{k} + a_2\tilde{k}^2 + a_3\tilde{k}^3) > 0$ for any $\tilde{k} < \tilde{k}_0$.

In summary, for any parameter choice in the chosen parameter region, since $a_0 + a_1\tilde{k}_0 + a_2\tilde{k}_0^2 + a_3\tilde{k}_0^3 < 0$ and $\frac{d}{d\tilde{k}}(a_0 + a_1\tilde{k} + a_2\tilde{k}^2 + a_3\tilde{k}^3) > 0$ for any $\tilde{k} < \tilde{k}_0$, we have $a_0 + a_1\tilde{k} + a_2\tilde{k}^2 + a_3\tilde{k}^3 < 0$ for any $\tilde{k} < \tilde{k}_0$.

Therefore, all $\tilde{k}$ solutions of $a_0 + a_1\tilde{k} + a_2\tilde{k}^2 + a_3\tilde{k}^3 = 0$ in the chosen parameter region are larger than $\tilde{k}_0 \equiv -\frac{b_0}{b_1}$.

**End Of Proof.**

It means the number of TPs is only determined by the number of roots of $a_0 + a_1(ka) + a_2(ka)^2 + a_3(ka)^3 = 0$ for our choices of parameters. For convenience, we define following parameters:

$$\begin{aligned}\eta &= 18a_0a_1a_2a_3 - 4a_2^3a_0 + a_2^2a_1^2 - 4a_3a_1^3 - 27a_3^2a_0^2\\ \eta_0 &= a_2^2 - 3a_3a_1\end{aligned} \tag{17}$$

It turns out, in the chosen parameter region,
(i) if $\eta < 0$, and there is only one root, which means there are two TPs on one $C_3$ axis;
(ii)if $\eta = 0$ and $\eta_0 \neq 0$, there are one single root and one double root, which means there are four TPs on one $C_3$ axist;
(iii)if $\eta > 0$ and there are three roots, which means there are six TPs on one $C_3$ axis;
(iv) $\eta = 0$ and $\eta_0 = 0$ doesn't exist.

Those give the phase diagram shown in Fig.1g.

## III. Kane Model Parameter Choices for Surface States

| $\frac{E_c}{\varepsilon_0}$ | $\frac{E_v}{\varepsilon_0}$ | $\gamma_1$ | $\gamma_2$ | $\gamma_3$ | $\frac{C}{\beta_c/a}$ | $\frac{P}{\beta_c/a}$ | $B_{8v}^+/\beta_c$ | $B_{8v}^-/\beta_c$ |
|---|---|---|---|---|---|---|---|---|
| $-2$ | 0 | 2 | $-1$ | 0.5 | $-0.15$ | 2.5 | 0 | 0 |

TABLE II. Choices of Kane model parameters for Fig.3a with 2 TPs on one $C_3$ axis.

| $\frac{E_c}{\varepsilon_0}$ | $\frac{E_v}{\varepsilon_0}$ | $\gamma_1$ | $\gamma_2$ | $\gamma_3$ | $\frac{C}{\beta_c/a}$ | $\frac{P}{\beta_c/a}$ | $B_{8v}^+/\beta_c$ | $B_{8v}^-/\beta_c$ |
|---|---|---|---|---|---|---|---|---|
| $-3$ | 0 | 2 | $-1$ | 0.5 | $-0.05$ | 2.5 | 0 | 0 |

TABLE III. Choices of Kane model parameters for Fig.3b with 6 TPs on one $C_3$ axis.

## IV. Crystal structure and bands structure of LuPtBi, LuAuPb and LuPdBi

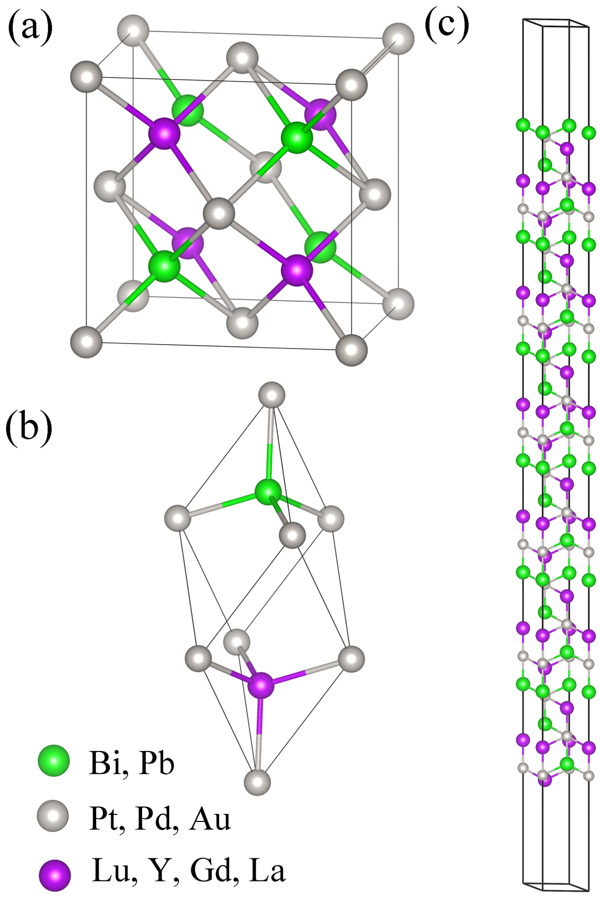


FIG. S1. Crystal structure of the calculated half-Heusler compounds. (a) unitcell, (b) primitive cell and (c) slab structure.

## V. *Ab inito* calculations of surface states for YPtBi and LaPtBi.

The electronic ground states of these half Heusler compounds were calculated by using density-functional theory (DFT) within the Perdew-Burke-Ernzerhof-type generalized-gradient approximation (GGA)[10] using the Vienna *ab initio* Simulation Package (VASP)[11]. For the bulk materials calculation, primitive cells with experimental crystal parameters were selected as shown in Fig.S1(b). In order to get an accurate fermi energy, a dense k points with the mesh grid 21 × 21 × 1 was utilized in each static calculation. To calculate the surface state, a slab, exposing (111) plane of the FCC structure, with 54 atom layers (around 60 $\AA$) and 20 $\AA$ vacuum thickness was used for each material, as shown in Fig.S1(c). In the slab calculation, a 10 × 10 × 1 k points mesh grid for static calculation and 51 × 51 × 1 k points mesh grid for fermi surface calculation were utilized. While calculating the surface state dispersion and fermi surface of YPtBi and LaPtBi, the upmost 9 atom layers which are terminated by Bi(Pb) atoms are considered as surface atoms. Spin-orbit coupling (SOC) was included in all calculations.

---

* binghai.yan@weizmann.ac.il

1 P. C. Canfield, J. Thompson, W. Beyermann, A. Lacerda, M. Hundley, E. Peterson, Z. Fisk, and H. Ott, Journal of applied physics **70**, 5800 (1991).

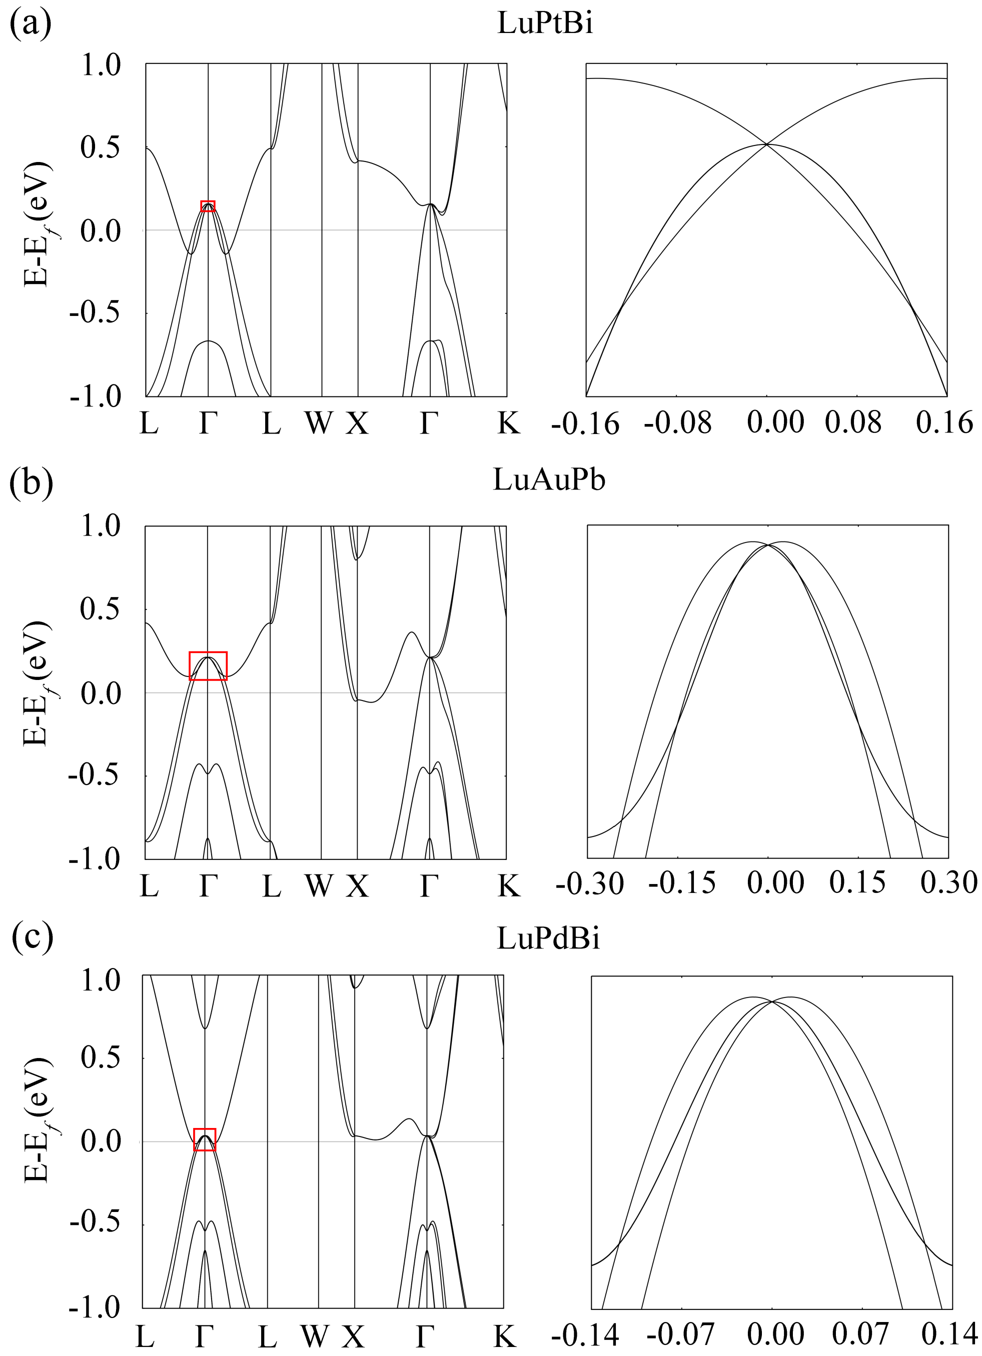


FIG. S2. Bulk band structures with triply degenerate band crossing. All these three materials are long-TP materials, holding different numbers of TPs: (a) LuPtBi with 6 TPs along the C3 axis, (b) LuAuPb with 6 TPs, and (c) LaPtBi with 2 TPs. To make it more clear, the band dispersion along the C3 axis in the red boxes are zoomed-in and shown in corresponding right panels.

[2] M. I. Aroyo, J. M. Perez-Mato, C. Capillas, E. Kroumova, S. Ivantchev, G. Madariaga, A. Kirov, and H. Wondratschek, Zeitschrift für Kristallographie-Crystalline Materials **221**, 15 (2006).

[3] R. Winkler, S. Papadakis, E. De Poortere, and M. Shayegan, *Spin-Orbit Coupling in Two-Dimensional Electron and Hole Systems*, Vol. 41 (Springer, 2003).

[4] H. Lin, L. A. Wray, Y. Xia, S. Xu, S. Jia, R. J. Cava, A. Bansil, and M. Z. Hasan, Nature materials **9**, 546 (2010).

[5] S. Chadov, X. Qi, J. Kübler, G. H. Fecher, C. Felser, and S. C. Zhang, Nature materials **9**, 541 (2010).

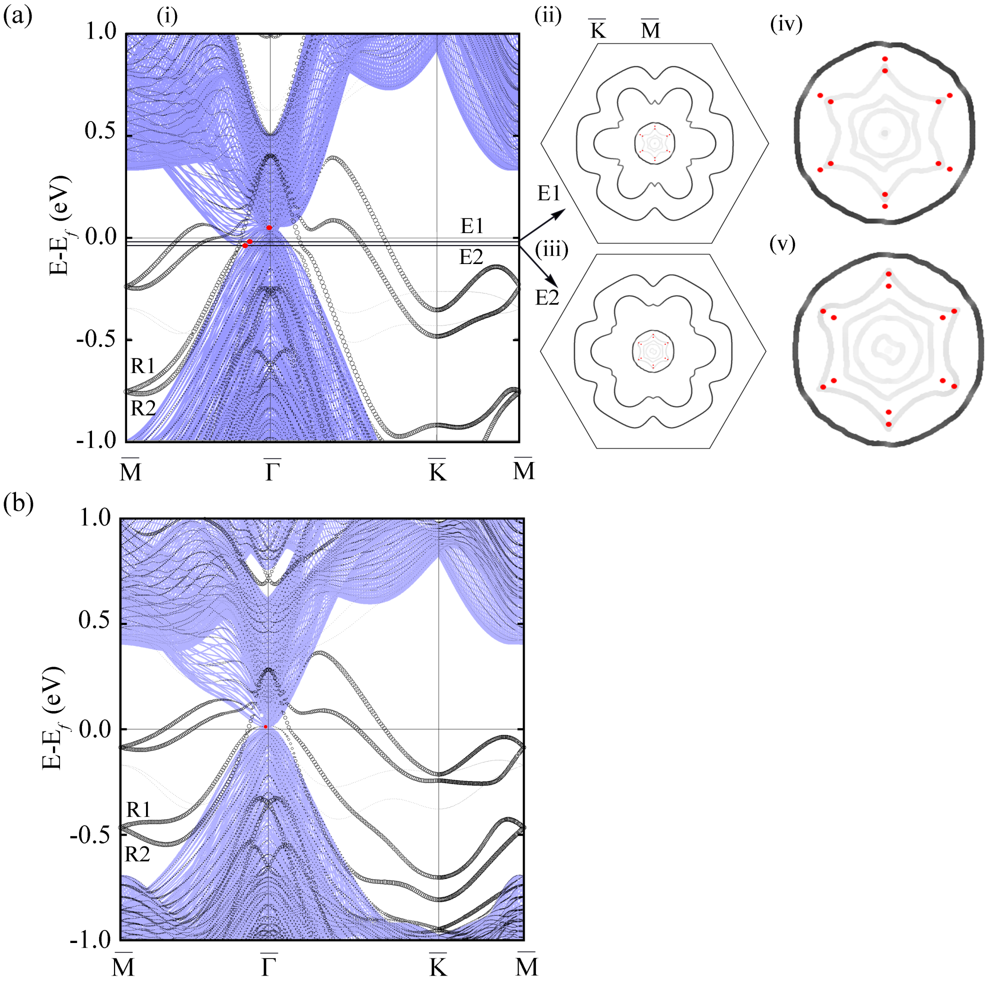


FIG. S3. The DFT surface band structures calculated on slab models for (a) YPtBi and (b) LaPtBi. The size of white circles represent the surface contribution and thus large circles indicate the surface states. The bulk bands are indicated by blue curves as a background, where the triple point is indicated by the red point. (ii) and (iii), Fermi surfaces corresponding to energy E1 (crossing the triple point) and E2(crossing the triple point), respectively. (iv) and (v), The zoom-in of the inner Fermi ring of (ii) and (iii), respectively. For YPtBi, at each energy level Fermi arcs connect 6 TPs and form a hexagon-like Fermi surface, consistent with the Kane model. In both cases, the Rashba-like surface states R1 and R2 exists and R1 end at the TPs, similar with that of GdPtBi Fig.3(c).

[6] D. Xiao, Y. Yao, W. Feng, J. Wen, W. Zhu, X.-Q. Chen, G. M. Stocks, and Z. Zhang, Phys. Rev. Lett. **105**, 096404 (2010).
[7] W. Al-Sawai, H. Lin, R. S. Markiewicz, L. A. Wray, Y. Xia, S.-Y. Xu, M. Z. Hasan, and A. Bansil, Phys. Rev. B **82**, 125208 (2010).
[8] Z. Zhu, G. W. Winkler, Q. Wu, J. Li, and A. A. Soluyanov, Phys. Rev. X **6**, 031003 (2016).
[9] G. Burns, *Introduction to group theory with applications: materials science and technology* (Academic Press, 2014).
[10] J. P. Perdew, K. Burke, and M. Ernzerhof, Phys. Rev. Lett. **77**, 3865 (1996).
[11] G. Kresse and J. Furthmüller, Comp. Mater. Sci. **6**, 15 (1996).
